# Supplementary material for: Skeptic: Automatic, Justified and Privacy-Preserving Password Composition Policy Selection
Source: arXiv:2007.03809 source file (2024-03-15)
Supplement: Supplementary file 1 [file _appendices.tex]

\section{Experimental data: Shay et al.}
The following results were produced for each dataset. Rankings produced by Skeptic under each selection mode (heading ``Skeptic'') are compared to those by Shay et al. \cite{shay2016designing} (heading ``Shay'') at $10^{14}$ guesses. Power-law curve $\alpha$ values given (heading ``$\alpha$'', as well as distance between our rankings and previous results (heading ``Distance''). Mean pairwise ranking distance ($mprd$) is given for each to give an idea of overall agreement and is computed by averaging the distance column.

\subsection{Yahoo}
The following results produced by Pyrrho from the Yahoo dataset. 

\begin{table}[H] \label{tbl:a-yahoo-prop}
\centering
\caption{Policy rankings produced under proportional reselection.}
\begin{tabular}{|l|l|l|l|l|}
\hline
Policy   & Shay & Skeptic & $\alpha$ & Distance \\ \hline
3class16 & 1    & 1       & -0.15000 & 0        \\ \hline % -0.150000001833355
basic20  & 2    & 3       & -0.22732 & 1        \\ \hline % -0.22731830236841
2word16  & 3    & 2       & -0.18900 & 1        \\ \hline % -0.188997503044491
basic16  & 4    & 7       & -0.45304 & 3        \\ \hline % -0.45303574888882
3class12 & 5    & 4       & -0.28309 & 1        \\ \hline % -0.283097964529562
2word12  & 6    & 6       & -0.31745 & 0        \\ \hline % -0.317451317379454
comp8    & 7    & 5       & -0.29652 & 2        \\ \hline % -0.296523485604993
basic12  & 8    & 8       & -0.47954 & 0        \\ \hline % -0.479541875046041
\end{tabular}
\begin{equation*}
    mprd=1
\end{equation*}
\end{table}

\begin{table}[H]
\centering
\caption{Policy rankings produced under convergent reselection.}
\begin{tabular}{|l|l|l|l|l|}
\hline
Policy   & Shay & Skeptic & $\alpha$ & Distance \\ \hline
3class16 & 1    & 7       & -1.33182 & 6        \\ \hline % -1.3318152699160488
basic20  & 2    & 8       & -1.65587 & 6        \\ \hline % -1.6558723484160862
2word16  & 3    & 6       & -1.33178 & 3        \\ \hline % -1.3317786933594493
basic16  & 4    & 5       & -1.02369 & 1        \\ \hline % -1.0236920667679512
3class12 & 5    & 2       & -0.77450 & 3        \\ \hline % -0.7745013924378557
2word12  & 6    & 3       & -0.82019 & 3        \\ \hline % -0.8201873276216698
comp8    & 7    & 4       & -0.87005 & 3        \\ \hline % -0.8700493666798914
basic12  & 8    & 1       & -0.77239 & 7        \\ \hline % -0.7723873654120519
\end{tabular}
\begin{equation*}
    mprd=4
\end{equation*}
\end{table}

\begin{table}[H]
\centering
\caption{Policy rankings produced under extraneous reselection.}
\begin{tabular}{|l|l|l|l|l|}
\hline
Policy   & Shay & Skeptic & $\alpha$ & Distance \\ \hline
3class16 & 1    & 1       & -0.04211 & 0        \\ \hline % -0.04210526402632619
basic20  & 2    & 4       & -0.05134 & 2        \\ \hline % -0.05134151255309264
2word16  & 3    & 2       & -0.05134 & 1        \\ \hline % -0.05134151255309264
basic16  & 4    & 6       & -0.17558 & 2        \\ \hline % -0.17558403806147313
3class12 & 5    & 5       & -0.15869 & 0        \\ \hline % -0.15869415660817537
2word12  & 6    & 7       & -0.18670 & 1        \\ \hline % -0.18670016935807232
comp8    & 7    & 3       & -0.15048 & 4        \\ \hline % -0.15048415667165857
basic12  & 8    & 8       & -0.35504 & 0        \\ \hline % -0.35504148566217963
\end{tabular}
\begin{equation*}
    mprd=1.25
\end{equation*}
\end{table}

\begin{table}[H]
\centering
\caption{Policy rankings produced under null reselection.}
\begin{tabular}{|l|l|l|l|l|}
\hline
Policy   & Shay & Skeptic & $\alpha$ & Distance \\ \hline
3class16 & 1    & 1       & -0.00016 & 0        \\ \hline % -0.00015790845114059846
basic20  & 2    & 2       & -0.00017 & 0        \\ \hline % -0.0001748125629368484
2word16  & 3    & 3       & -0.00034 & 0        \\ \hline % -0.0003444676692301792
basic16  & 4    & 6       & -0.01238 & 2        \\ \hline % -0.012379177947589803
3class12 & 5    & 5       & -0.00946 & 0        \\ \hline % -0.009464853216191964
2word12  & 6    & 7       & -0.01360 & 1        \\ \hline % -0.013602453430650915
comp8    & 7    & 4       & -0.00620 & 3        \\ \hline % -0.006197599482015045
basic12  & 8    & 8       & -0.16874 & 0        \\ \hline % -0.16874098618285094
\end{tabular}
\begin{equation*}
    mprd=0.75
\end{equation*}
\end{table}

\subsection{RockYou}
The following results produced by Pyrrho from the RockYou dataset.

\begin{table}[H]
\centering
\caption{Policy rankings produced under proportional reselection.}
\begin{tabular}{|l|l|l|l|l|}
\hline
Policy   & Shay & Skeptic & $\alpha$ & Distance \\ \hline
3class16 & 1    & 1       & -0.32803 & 0        \\ \hline % -0.328031837920168
basic20  & 2    & 4       & -0.45407 & 2        \\ \hline % -0.454074299827686
2word16  & 3    & 3       & -0.43460 & 0        \\ \hline % -0.434602888404911
basic16  & 4    & 7       & -0.57962 & 3        \\ \hline % -0.579615909000248
3class12 & 5    & 2       & -0.33753 & 3        \\ \hline % -0.337533847665868
2word12  & 6    & 5       & -0.49108 & 1        \\ \hline % -0.491081508483271
comp8    & 7    & 6       & -0.54964 & 1        \\ \hline % -0.549638759867585
basic12  & 8    & 8       & -0.58639 & 0        \\ \hline % -0.586394707428606
\end{tabular}
\begin{equation*}
    mprd=1.25
\end{equation*}
\end{table}

\begin{table}[H]
\centering
\caption{Policy rankings produced under convergent reselection.}
\begin{tabular}{|l|l|l|l|l|}
\hline
Policy   & Shay & Skeptic & $\alpha$ & Distance \\ \hline
3class16 & 1    & 2       & -0.73706 & 1        \\ \hline % -0.7370600303865892
basic20  & 2    & 7       & -0.86310 & 5        \\ \hline % -0.8631044205311791
2word16  & 3    & 5       & -0.79623 & 2        \\ \hline % -0.7962302362383675
basic16  & 4    & 6       & -0.85714 & 2        \\ \hline % -0.8571363235418632
3class12 & 5    & 1       & -0.66272 & 4        \\ \hline % -0.6627194044723481
2word12  & 6    & 3       & -0.74833 & 3        \\ \hline % -0.7483331444938627
comp8    & 7    & 8       & -0.92870 & 1        \\ \hline % -0.9286992229097784
basic12  & 8    & 4       & -0.77957 & 4        \\ \hline % -0.7795740115228937
\end{tabular}
\begin{equation*}
    mprd=2.75
\end{equation*}
\end{table}

\begin{table}[H]
\centering
\caption{Policy rankings produced under extraneous reselection.}
\begin{tabular}{|l|l|l|l|l|}
\hline
Policy   & Shay & Skeptic & $\alpha$ & Distance \\ \hline
3class16 & 1    & 1       & -0.17322 & 0        \\ \hline % -0.1732211425958675
basic20  & 2    & 3       & -0.24107 & 1        \\ \hline % -0.241065664695532
2word16  & 3    & 4       & -0.24636 & 1        \\ \hline % -0.24636409010032567
basic16  & 4    & 7       & -0.38191 & 3        \\ \hline % -0.3819146716743862
3class12 & 5    & 2       & -0.22171 & 3        \\ \hline % -0.22171184178758788
2word12  & 6    & 6       & -0.35128 & 0        \\ \hline % -0.3512831245013512
comp8    & 7    & 5       & -0.29032 & 2        \\ \hline % -0.29031771828970143
basic12  & 8    & 8       & -0.49859 & 0        \\ \hline % -0.49858696194583363
\end{tabular}
\begin{equation*}
    mprd=1.25
\end{equation*}
\end{table}

\begin{table}[H]
\centering
\caption{Policy rankings produced under null reselection.}
\begin{tabular}{|l|l|l|l|l|}
\hline
Policy   & Shay & Skeptic & $\alpha$ & Distance \\ \hline
3class16 & 1    & 1       & -0.00481 & 0        \\ \hline % -0.004809677968672
basic20  & 2    & 2       & -0.00774 & 0        \\ \hline % -0.007736129787373
2word16  & 3    & 3       & -0.01311 & 0        \\ \hline % -0.013105260705404
basic16  & 4    & 7       & -0.11203 & 3        \\ \hline % -0.112034361640235
3class12 & 5    & 5       & -0.01818 & 0        \\ \hline % -0.018181608224376
2word12  & 6    & 6       & -0.07942 & 0        \\ \hline % -0.079421729135592
comp8    & 7    & 4       & -0.01573 & 3        \\ \hline % -0.015733457331725
basic12  & 8    & 8       & -0.32090 & 0        \\ \hline % -0.320900187849602
\end{tabular}
\begin{equation*}
    mprd=0.75
\end{equation*}
\end{table}

\subsection{LinkedIn}
The following results produced by Pyrrho from the LinkedIn dataset. 

\begin{table}[H]
\centering
\caption{Policy rankings produced under proportional reselection.}
\begin{tabular}{|l|l|l|l|l|}
\hline
Policy   & Shay & Skeptic & $\alpha$ & Distance \\ \hline
3class16 & 1    & 2       & -0.45101 & 1        \\ \hline % -0.4510142240235451
basic20  & 2    & 1       & -0.45052 & 1        \\ \hline % -0.4505241513185305
2word16  & 3    & 3       & -0.52490 & 0        \\ \hline % -0.5248958537542961
basic16  & 4    & 4       & -0.57100 & 0        \\ \hline % -0.5709974791941261
3class12 & 5    & 5       & -0.58018 & 0        \\ \hline % -0.5801754605463195
2word12  & 6    & 7       & -0.61491 & 1        \\ \hline % -0.6149086458490779
comp8    & 7    & 8       & -0.65135 & 1        \\ \hline % -0.6513514086846621
basic12  & 8    & 6       & -0.59159 & 2        \\ \hline % -0.59158613933814
\end{tabular}
\begin{equation*}
    mprd=0.75
\end{equation*}
\end{table}

\begin{table}[H]
\centering
\caption{Policy rankings produced under convergent reselection.}
\begin{tabular}{|l|l|l|l|l|}
\hline
Policy   & Shay & Skeptic & $\alpha$ & Distance \\ \hline
3class16 & 1    & 5       & -0.84807 & 4        \\ \hline % -0.8480745130620257
basic20  & 2    & 8       & -0.90303 & 6        \\ \hline % -0.9030320987318488
2word16  & 3    & 7       & -0.89905 & 4        \\ \hline % -0.899054755355177
basic16  & 4    & 3       & -0.79663 & 1        \\ \hline % -0.7966304699343845
3class12 & 5    & 2       & -0.77998 & 3        \\ \hline % -0.7799770935688873
2word12  & 6    & 4       & -0.83476 & 2        \\ \hline % -0.8347560109312953
comp8    & 7    & 6       & -0.84855 & 1        \\ \hline % -0.8485486697681716
basic12  & 8    & 1       & -0.73119 & 7        \\ \hline % -0.7311926960896533
\end{tabular}
\begin{equation*}
    mprd=3.5
\end{equation*}
\end{table}

\begin{table}[H]
\centering
\caption{Policy rankings produced under extraneous reselection.}
\begin{tabular}{|l|l|l|l|l|}
\hline
Policy   & Shay & Skeptic & $\alpha$ & Distance \\ \hline
3class16 & 1    & 2       & -0.25849 & 1        \\ \hline % -0.258487667311501
basic20  & 2    & 1       & -0.24783 & 1        \\ \hline % -0.2478302856974191
2word16  & 3    & 3       & -0.29777 & 0        \\ \hline % -0.2977719578887627
basic16  & 4    & 4       & -0.40212 & 0        \\ \hline % -0.4021997188377
3class12 & 5    & 6       & -0.43334 & 1        \\ \hline % -0.43333756896014186
2word12  & 6    & 5       & -0.42870 & 1        \\ \hline % -0.4286963998704655
comp8    & 7    & 7       & -0.45946 & 0        \\ \hline % -0.4594561194976184
basic12  & 8    & 8       & -0.53008 & 0        \\ \hline % -0.5300844001874699
\end{tabular}
\begin{equation*}
    mprd=0.5
\end{equation*}
\end{table}

\begin{table}[H]
\centering
\caption{Policy rankings produced under null reselection.}
\begin{tabular}{|l|l|l|l|l|}
\hline
Policy   & Shay & Skeptic & $\alpha$ & Distance \\ \hline
3class16 & 1    & 2       & -0.00512 & 1        \\ \hline % -0.005119700140876735
basic20  & 2    & 1       & -0.00207 & 1        \\ \hline % -0.002065442726884162
2word16  & 3    & 3       & -0.01272 & 0        \\ \hline % -0.01271757597379048
basic16  & 4    & 4       & -0.11099 & 0        \\ \hline % -0.11099256296522678
3class12 & 5    & 6       & -0.18384 & 1        \\ \hline % -0.1838419851528793
2word12  & 6    & 5       & -0.17379 & 1        \\ \hline % -0.17379245774700025
comp8    & 7    & 7       & -0.21988 & 0        \\ \hline % -0.2198828897383922
basic12  & 8    & 8       & -0.44626 & 0        \\ \hline % -0.44625701958531794
\end{tabular}
\begin{equation*}
    mprd=0.5
\end{equation*}
\end{table}

\section{Replication results: Shay et al.}
The following scatter plots show the correlation between the $\alpha$ values of power-law equations fitted to proportional (average case) reselection results produced by \textit{Skeptic} and the rankings empirically determined by Shay et al. in \cite{shay2016designing}. Each plot is annotated with its Pearson correlation coefficient $\rho$.

\subsection{Yahoo}
\begin{figure}[H]
    \centering
    \includegraphics[width=0.9\columnwidth]{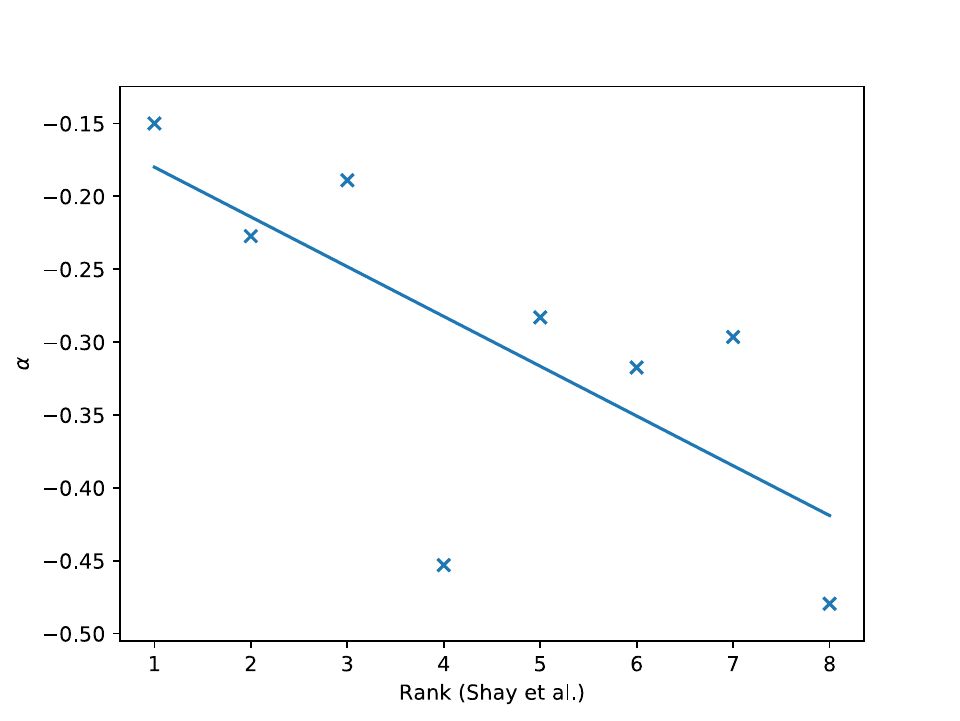}
    \caption{Proportional reselection.}
    \label{fig:my_label_1}
    \begin{equation*}
        \rho=-0.7128752913482401
    \end{equation*}
\end{figure}

\subsection{RockYou}
\begin{figure}[H]
    \centering
    \includegraphics[width=0.9\columnwidth]{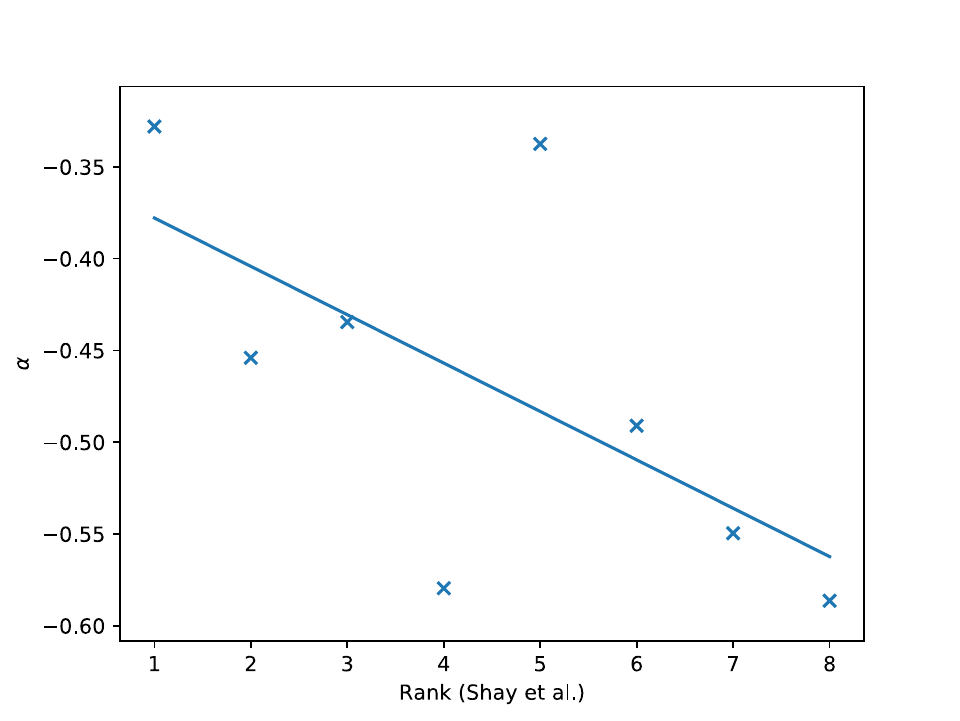}
    \caption{Proportional reselection.}
    \label{fig:my_label_2}
    \begin{equation*}
        \rho=-0.6384628682993778
    \end{equation*}
\end{figure}

\subsection{LinkedIn}
\begin{figure}[H]
    \centering
    \includegraphics[width=0.9\columnwidth]{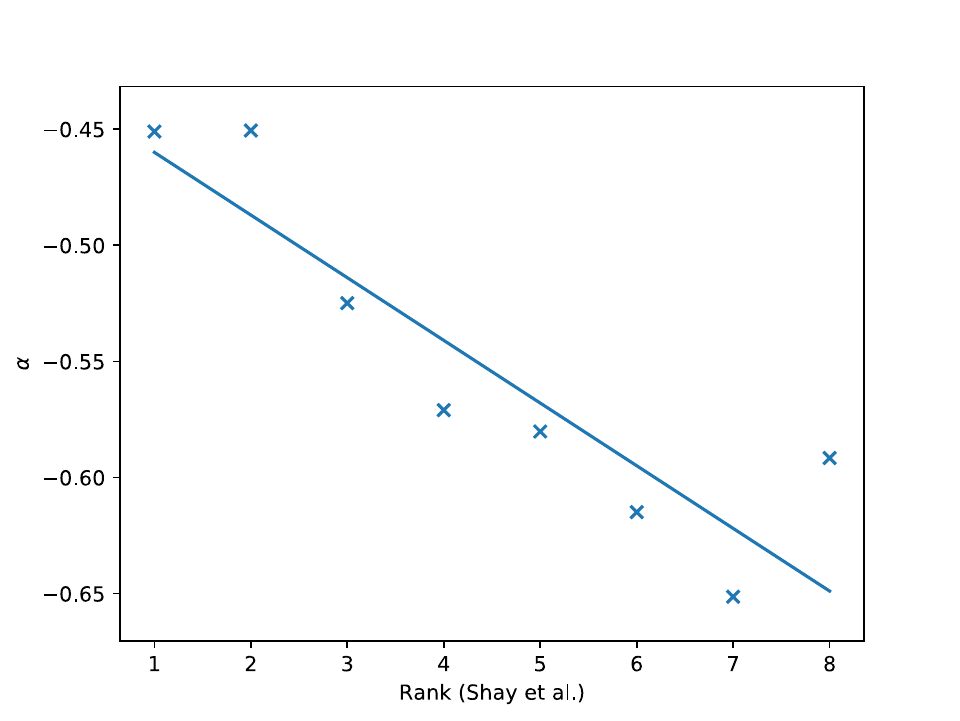}
    \caption{Proportional reselection.}
    \label{fig:my_label_3}
    \begin{equation*}
        \rho=-0.9005449627393818
    \end{equation*}
\end{figure}

\section{Experimental data: Weir et al.}

\begin{table}[H]
\centering
\caption{Yahoo proportional}
\begin{tabular}{|l|l|l|l|l|}
\hline
Policy   & Weir & Skeptic & $\alpha$ & Distance \\ \hline
symbol10 & 1    & 2       & -0.32002 & 1        \\ \hline % -0.320019090237718
symbol9  & 2    & 1       & -0.29548 & 1        \\ \hline % -0.295475843288516
symbol8  & 3    & 7       & -0.35748 & 4        \\ \hline % -0.357477064159878
upper10  & 4    & 5       & -0.33300 & 1        \\ \hline % -0.332996715456861
symbol7  & 5    & 8       & -0.41519 & 3        \\ \hline % -0.415192888759335
upper9   & 6    & 4       & -0.33151 & 2        \\ \hline % -0.331512666495103
upper8   & 7    & 6       & -0.34709 & 1        \\ \hline % -0.34708686659925
upper7   & 8    & 3       & -0.32624 & 5        \\ \hline % -0.326237545968052
basic10  & 9    & 9       & -0.48500 & 0        \\ \hline % -0.485004346203473
basic9   & 10   & 10      & -0.49911 & 0        \\ \hline % -0.499108167959326
basic8   & 11   & 12      & -0.56605 & 1        \\ \hline % -0.566051941104415
basic7   & 12   & 11      & -0.56231 & 1        \\ \hline % -0.562306050086818
\end{tabular}
\begin{equation*}
    mprd=1.67 % 1.66666666666667
\end{equation*}
\end{table}

\begin{table}[H]
\centering
\caption{Yahoo convergent}
\begin{tabular}{|l|l|l|l|l|}
\hline
Policy   & Weir & Skeptic & $\alpha$ & Distance \\ \hline
symbol10 & 1    & 12      & -0.81123 & 11       \\ \hline % -0.811227798800374
symbol9  & 2    & 8       & -0.72096 & 6        \\ \hline % -0.720963029089251
symbol8  & 3    & 10      & -0.76600 & 7        \\ \hline % -0.765999572114918
upper10  & 4    & 9       & -0.75269 & 5        \\ \hline % -0.752686181848347
symbol7  & 5    & 11      & -0.78870 & 6        \\ \hline % -0.788700654817024
upper9   & 6    & 4       & -0.68842 & 2        \\ \hline % -0.688419067420068
upper8   & 7    & 6       & -0.70280 & 1        \\ \hline % -0.702796687770826
upper7   & 8    & 1       & -0.63983 & 7        \\ \hline % -0.63983100467906
basic10  & 9    & 7       & -0.70883 & 2        \\ \hline % -0.708832661734246
basic9   & 10   & 3       & -0.67839 & 7        \\ \hline % -0.678388765092003
basic8   & 11   & 5       & -0.69848 & 6        \\ \hline % -0.698480480512314
basic7   & 12   & 2       & -0.66790 & 10       \\ \hline % -0.667901363570134
\end{tabular}
\begin{equation*}
    mprd=5.83 % 5.83333333333333
\end{equation*}
\end{table}

\begin{table}[H]
\centering
\caption{Yahoo extraneous}
\begin{tabular}{|l|l|l|l|l|}
\hline
Policy   & Weir & Skeptic & $\alpha$ & Distance \\ \hline
symbol10 & 1    & 1       & -0.18744 & 0        \\ \hline % -0.187442966703073
symbol9  & 2    & 2       & -0.19155 & 0        \\ \hline % -0.19154796592903
symbol8  & 3    & 4       & -0.23556 & 1        \\ \hline % -0.23555861985848
upper10  & 4    & 3       & -0.22055 & 1        \\ \hline % -0.220554417524206
symbol7  & 5    & 8       & -0.27091 & 3        \\ \hline % -0.270907280037943
upper9   & 6    & 5       & -0.24554 & 1        \\ \hline % -0.245536024258508
upper8   & 7    & 6       & -0.26689 & 1        \\ \hline % -0.266894897049293
upper7   & 8    & 7       & -0.26689 & 1        \\ \hline % -0.266894897049293
basic10  & 9    & 9       & -0.43376 & 0        \\ \hline % -0.43376475498875
basic9   & 10   & 10      & -0.47508 & 0        \\ \hline % -0.475078293960674
basic8   & 11   & 11      & -0.54362 & 0        \\ \hline % -0.543615417117954
basic7   & 12   & 12      & -0.56231 & 0        \\ \hline % -0.562306050881446
\end{tabular}
\begin{equation*}
    mprd=0.67 % 0.666666666666667
\end{equation*}
\end{table}

\begin{table}[H]
\centering
\caption{Yahoo null}
\begin{tabular}{|l|l|l|l|l|}
\hline
Policy   & Weir & Skeptic & $\alpha$ & Distance \\ \hline
symbol10 & 1    & 1       & -0.01556 & 0        \\ \hline % -0.015564167473273
symbol9  & 2    & 2       & -0.01887 & 0        \\ \hline % -0.018871220622022
symbol8  & 3    & 4       & -0.03759 & 1        \\ \hline % -0.037592310964835
upper10  & 4    & 3       & -0.03321 & 1        \\ \hline % -0.033205695796485
symbol7  & 5    & 6       & -0.06282 & 1        \\ \hline % -0.062818164211923
upper9   & 6    & 5       & -0.05096 & 1        \\ \hline % -0.050956596285808
upper8   & 7    & 8       & -0.08789 & 1        \\ \hline % -0.087885338307444
upper7   & 8    & 7       & -0.08667 & 1        \\ \hline % -0.086671352731622
basic10  & 9    & 9       & -0.32446 & 0        \\ \hline % -0.324458546763458
basic9   & 10   & 10      & -0.39767 & 0        \\ \hline % -0.397667944294436
basic8   & 11   & 11      & -0.52440 & 0        \\ \hline % -0.524401090971686
basic7   & 12   & 12      & -0.54077 & 0        \\ \hline % -0.540768194296323
\end{tabular}
\begin{equation*}
    mprd=0.5
\end{equation*}
\end{table}

\begin{table}[H]
\centering
\caption{RockYou proportional}
\begin{tabular}{|l|l|l|l|l|}
\hline
Policy   & Weir & Skeptic & $\alpha$ & Distance \\ \hline
symbol10 & 1    & 3       & -0.55159 & 2        \\ \hline % -0.551590464244535
symbol9  & 2    & 4       & -0.58810 & 2        \\ \hline % -0.588098630934787
symbol8  & 3    & 7       & -0.61414 & 4        \\ \hline % -0.61413717745509
upper10  & 4    & 1       & -0.51254 & 3        \\ \hline % -0.51253601635051
symbol7  & 5    & 5       & -0.60034 & 0        \\ \hline % -0.600338690489993
upper9   & 6    & 2       & -0.55140 & 4        \\ \hline % -0.551404671084113
upper8   & 7    & 8       & -0.61888 & 1        \\ \hline % -0.618883001691848
upper7   & 8    & 6       & -0.60294 & 2        \\ \hline % -0.60293509146904
basic10  & 9    & 9       & -0.67358 & 0        \\ \hline % -0.673580606619615
basic9   & 10   & 10      & -0.74060 & 0        \\ \hline % -0.74059964193201
basic8   & 11   & 11      & -0.75840 & 0        \\ \hline % -0.75839599758178
basic7   & 12   & 12      & -0.76364 & 0        \\ \hline % -0.763643560370707
\end{tabular}
\begin{equation*}
    mprd=1.5
\end{equation*}
\end{table}

\begin{table}[H]
\centering
\caption{RockYou convergent}
\begin{tabular}{|l|l|l|l|l|}
\hline
Policy   & Weir & Skeptic & $\alpha$ & Distance \\ \hline
symbol10 & 1    & 6       & -0.80188 & 5        \\ \hline % -0.801875957547684
symbol9  & 2    & 4       & -0.79545 & 2        \\ \hline % -0.795454891822942
symbol8  & 3    & 8       & -0.82135 & 5        \\ \hline % -0.821354821404331
upper10  & 4    & 1       & -0.78038 & 3        \\ \hline % -0.780381961709881
symbol7  & 5    & 7       & -0.80743 & 2        \\ \hline % -0.807434593778842
upper9   & 6    & 2       & -0.78159 & 4        \\ \hline % -0.781585945960103
upper8   & 7    & 9       & -0.82309 & 2        \\ \hline % -0.823085069851623
upper7   & 8    & 3       & -0.78834 & 5        \\ \hline % -0.788341785033446
basic10  & 9    & 5       & -0.79945 & 4        \\ \hline % -0.799454426413728
basic9   & 10   & 10      & -0.82980 & 0        \\ \hline % -0.829804401209344
basic8   & 11   & 12      & -0.83558 & 1        \\ \hline % -0.8355842499383
basic7   & 12   & 11      & -0.83373 & 1        \\ \hline % -0.833734273371648
\end{tabular}
\begin{equation*}
    mprd=2.83 % 2.83333333333333
\end{equation*}
\end{table}

\begin{table}[H]
\centering
\caption{RockYou extraneous}
\begin{tabular}{|l|l|l|l|l|}
\hline
Policy   & Weir & Skeptic & $\alpha$ & Distance \\ \hline
symbol10 & 1    & 2       & -0.40493 & 1        \\ \hline % -0.404927724373475
symbol9  & 2    & 4       & -0.46072 & 2        \\ \hline % -0.460721818409071
symbol8  & 3    & 5       & -0.48545 & 2        \\ \hline % -0.48544869139838
upper10  & 4    & 1       & -0.38164 & 3        \\ \hline % -0.381636077778196
symbol7  & 5    & 6       & -0.48818 & 1        \\ \hline % -0.488184082776828
upper9   & 6    & 3       & -0.44141 & 3        \\ \hline % -0.441409632719588
upper8   & 7    & 7       & -0.50596 & 0        \\ \hline % -0.505961148926222
upper7   & 8    & 8       & -0.52077 & 0        \\ \hline % -0.520772791592121
basic10  & 9    & 9       & -0.63137 & 0        \\ \hline % -0.631367204571857
basic9   & 10   & 10      & -0.70026 & 0        \\ \hline % -0.700264536092272
basic8   & 11   & 11      & -0.74041 & 0        \\ \hline % -0.740408621476455
basic7   & 12   & 12      & -0.74860 & 0        \\ \hline % -0.748597473549761
\end{tabular}
\begin{equation*}
    mprd=1
\end{equation*}
\end{table}

\begin{table}[H]
\centering
\caption{RockYou null}
\begin{tabular}{|l|l|l|l|l|}
\hline
Policy   & Weir & Skeptic & $\alpha$ & Distance \\ \hline
symbol10 & 1    & 2       & -0.15407 & 1        \\ \hline % -0.154070732249245
symbol9  & 2    & 4       & -0.22450 & 2        \\ \hline % -0.224503431772083
symbol8  & 3    & 5       & -0.26824 & 2        \\ \hline % -0.268238620492176
upper10  & 4    & 1       & -0.10831 & 3        \\ \hline % -0.108305992409738
symbol7  & 5    & 6       & -0.28506 & 1        \\ \hline % -0.285056407782036
upper9   & 6    & 3       & -0.18380 & 3        \\ \hline % -0.183796249244513
upper8   & 7    & 7       & -0.29844 & 0        \\ \hline % -0.298436168527346
upper7   & 8    & 8       & -0.31507 & 0        \\ \hline % -0.315068024766683
basic10  & 9    & 9       & -0.53300 & 0        \\ \hline % -0.533001823311373
basic9   & 10   & 10      & -0.64805 & 0        \\ \hline % -0.648050289801095
basic8   & 11   & 11      & -0.70358 & 0        \\ \hline % -0.703582448186162
basic7   & 12   & 12      & -0.73241 & 0        \\ \hline % -0.732412916718902
\end{tabular}
\begin{equation*}
    mprd=1
\end{equation*}
\end{table}

\begin{table}[H]
\centering
\caption{LinkedIn proportional}
\begin{tabular}{|l|l|l|l|l|}
\hline
Policy   & Weir & Skeptic & $\alpha$ & Distance \\ \hline
symbol10 & 1    & 2       & -0.59113 & 1        \\ \hline % -0.591125607565898
symbol9  & 2    & 1       & -0.57306 & 1        \\ \hline % -0.573062312278435
symbol8  & 3    & 3       & -0.63716 & 0        \\ \hline % -0.637160061538711
upper10  & 4    & 6       & -0.64463 & 2        \\ \hline % -0.644631998879243
symbol7  & 5    & 5       & -0.63890 & 0        \\ \hline % -0.63890220739714
upper9   & 6    & 7       & -0.64477 & 1        \\ \hline % -0.644771493436183
upper8   & 7    & 9       & -0.67203 & 2        \\ \hline % -0.672030599630624
upper7   & 8    & 8       & -0.66124 & 0        \\ \hline % -0.661240194459474
basic10  & 9    & 4       & -0.63873 & 5        \\ \hline % -0.638734067627644
basic9   & 10   & 10      & -0.68880 & 0        \\ \hline % -0.688795978953019
basic8   & 11   & 12      & -0.72456 & 1        \\ \hline % -0.724556525176091
basic7   & 12   & 11      & -0.71769 & 1        \\ \hline % -0.717691552183719
\end{tabular}
\begin{equation*}
    mprd=1.17 % 1.16666666666667
\end{equation*}
\end{table}

\begin{table}[H]
\centering
\caption{LinkedIn convergent}
\begin{tabular}{|l|l|l|l|l|}
\hline
Policy   & Weir & Skeptic & $\alpha$ & Distance \\ \hline
basic7   & 12   & 4       & -0.78039 & 8        \\ \hline % -0.780385300281843
basic8   & 11   & 7       & -0.79384 & 4        \\ \hline % -0.793844107137502
basic9   & 10   & 3       & -0.77558 & 7        \\ \hline % -0.77558016778182
basic10  & 9    & 1       & -0.74921 & 8        \\ \hline % -0.749209480818537
upper7   & 8    & 6       & -0.79011 & 2        \\ \hline % -0.790113699350695
upper8   & 7    & 11      & -0.81234 & 4        \\ \hline % -0.812340892955823
upper9   & 6    & 5       & -0.78643 & 1        \\ \hline % -0.786425446879901
symbol7  & 5    & 10      & -0.80207 & 5        \\ \hline % -0.802067042869362
upper10  & 4    & 12      & -0.81872 & 8        \\ \hline % -0.818723971577312
symbol8  & 3    & 9       & -0.80038 & 6        \\ \hline % -0.800376870527337
symbol9  & 2    & 2       & -0.75850 & 0        \\ \hline % -0.758496120268716
symbol10 & 1    & 8       & -0.79438 & 7        \\ \hline % -0.794380401470364
\end{tabular}
\begin{equation*}
    mprd=5
\end{equation*}
\end{table}

\begin{table}[H]
\centering
\caption{LinkedIn extraneous}
\begin{tabular}{|l|l|l|l|l|}
\hline
Policy   & Weir & Skeptic & $\alpha$ & Distance \\ \hline
symbol10 & 1    & 1       & -0.45380 & 0        \\ \hline % -0.453799878840267
symbol9  & 2    & 2       & -0.46565 & 0        \\ \hline % -0.465646796670343
symbol8  & 3    & 3       & -0.51610 & 0        \\ \hline % -0.516103963611644
upper10  & 4    & 5       & -0.53186 & 1        \\ \hline % -0.531863189414612
symbol7  & 5    & 4       & -0.51839 & 1        \\ \hline % -0.518388873565154
upper9   & 6    & 6       & -0.55852 & 0        \\ \hline % -0.558521132876959
upper8   & 7    & 7       & -0.59859 & 0        \\ \hline % -0.598592761398404
upper7   & 8    & 8       & -0.60101 & 0        \\ \hline % -0.601009738020508
basic10  & 9    & 9       & -0.60275 & 0        \\ \hline % -0.602754448078005
basic9   & 10   & 10      & -0.66974 & 0        \\ \hline % -0.66973846396697
basic8   & 11   & 12      & -0.71573 & 1        \\ \hline % -0.715732913437398
basic7   & 12   & 11      & -0.71214 & 1        \\ \hline % -0.7121449144858
\end{tabular}
\begin{equation*}
    mprd=0.33 % 0.333333333333333
\end{equation*}
\end{table}

\begin{table}[H]
\centering
\caption{LinkedIn null}
\begin{tabular}{|l|l|l|l|l|}
\hline
Policy   & Weir & Skeptic & $\alpha$ & Distance \\ \hline
symbol10 & 1    & 1       & -0.23443 & 0        \\ \hline % -0.234427453587019
symbol9  & 2    & 2       & -0.26074 & 0        \\ \hline % -0.260740493970895
symbol8  & 3    & 3       & -0.35575 & 0        \\ \hline % -0.355747988006753
upper10  & 4    & 4       & -0.35737 & 0        \\ \hline % -0.357367299269786
symbol7  & 5    & 5       & -0.36453 & 0        \\ \hline % -0.364526548309825
upper9   & 6    & 6       & -0.41293 & 0        \\ \hline % -0.412934580291385
upper8   & 7    & 8       & -0.50475 & 1        \\ \hline % -0.504746418395145
upper7   & 8    & 7       & -0.49261 & 1        \\ \hline % -0.492610064748683
basic10  & 9    & 9       & -0.55796 & 0        \\ \hline % -0.557956500420314
basic9   & 10   & 10      & -0.63726 & 0        \\ \hline % -0.637258050629719
basic8   & 11   & 11      & -0.69777 & 0        \\ \hline % -0.697771266850606
basic7   & 12   & 12      & -0.70531 & 0        \\ \hline % -0.705309373511038
\end{tabular}
\begin{equation*}
    mprd=0.17 % 0.166666666666667
\end{equation*}
\end{table}

\subsubsection{Frequencies to probabilities} It is straightforward to derive a password probability distribution from the input set. If we know the frequency with which a password occurs in the input set, and the total number of passwords it contains (its \textit{magnitude}) we can straightforwardly compute the probability that that password will permit access to a randomly-selected account on the system it originated from. 
Let a password frequency record in a representation of a user credential database $D$ originating from a system supporting password characters in set $S$ be a tuple $(s \in S^*, f \in \mathbb{N}, r \in \mathbb{N})$. Here $s$ is the password, which consists of some element in the set produced by applying the Kleene star operation to $S$, $f$ is the frequency with which $s$ appears in the database, and $r$ is the rank of the password in the database when ordered by frequency (that is, the most common password would have $r=1$, the second most common $r=2$ and so on). 
% Given a record $r=(s,f)$, we write $r_s$, $r_f$, to denote the elements $s$ and $f$ respectively. For example, if $r=(\textrm{`p4ss'},100)$, then $r_s=\textrm{`p4ss'}$, and $r_f=100$. 
The magnitude $mag(D)$ of a database $D$ represents the total number of passwords present on the system, and can readily be calculated by summing the frequency of each record together.

\begin{equation*}
    mag(D) = \sum_{(s, f, r) \in D}{} f
\end{equation*}

The set of password probability records of a database $D$ can be obtained by dividing the frequency of each record by the magnitude of $D$:

\begin{equation*}
    probs(D) = \{(s, \frac{f}{mag(D)}, r)  ~|~ (s, f, r) \in D\}
\end{equation*}

We call this newly-calculated probability $p$ (i.e. the second member of tuples in the set produced by $probs$). What we are left with is a probability distribution $P$ that will map passwords $s$ (outcomes) to the probability that a randomly-selected account on the system will have that password.

\begin{equation*}
    P(s) = 
    \begin{cases}
        p       & \text{if } (s, p, r) \in probs(D)\\
        0       & \text{otherwise}
    \end{cases}
\end{equation*}

We can plot the $r$ and $p$ of each tuple in $probs(D)$ as $x$ and $y$ coordinates respectively to visualise the \textit{rank-probability distribution} of $probs(D)$. Figure~\ref{fig:yahoo-basic6-scatter} shows a scatter plot of the rank-probability distribution of the Yahoo dataset used in this study. Note the log-log axes and the extremely long tail of the distribution made up of passwords with probabilities corresponding to frequencies in the low single digits. This is characteristic of a distribution of user-chosen passwords, with few passwords chosen very often and many passwords being chosen very rarely.

\begin{figure}[ht]
    \includegraphics[width=\columnwidth]{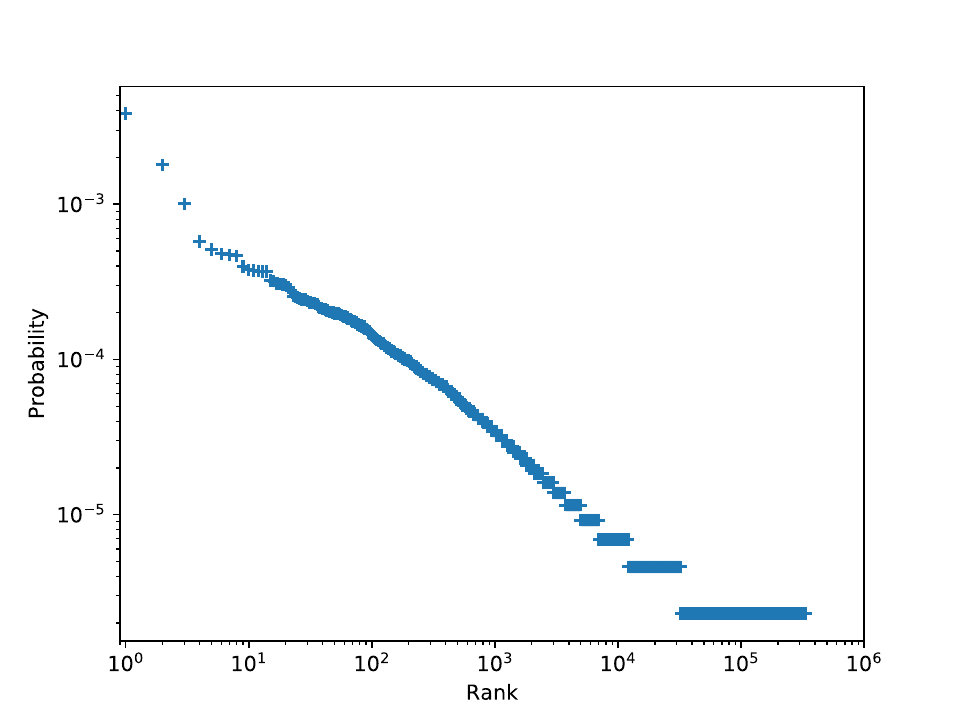}
    \caption{A scatter plot of the rank-probability distribution of passwords in the Yahoo dataset \cite{gross2012yahoo} used in this study.}
    \label{fig:yahoo-basic6-scatter}
\end{figure}

\begin{landscape}
  \begin{table}
    \centering
    \resizebox{\columnwidth}{!}{
      \begin{tabular}[c]{|*{16}{l|}}
        \hline
        & & \multirow{2}{*}{Policy} & \multicolumn{4}{c|}{Yahoo} & \multicolumn{4}{c|}{RockYou} & \multicolumn{4}{c|}{LinkedIn}\\
      \cline{4-15}
      & & & Shay & Skeptic & $\alpha$ & Distance & Shay & Skeptic & $\alpha$ & Distance & Shay & Skeptic & $\alpha$ & Distance\\
      \hline
      \multirow{32}{*}{\rotatebox{90}{Reselection modes}} & \multirow{8}{*}{\rotatebox{90}{Null}} & 3class16 & 1 & 1 & -0.00015790845 & 0 & 1 & 1 & -0.00480967797 & 0 & 1 & 2 & -0.00511970014 & 1\\
      \cline{3-15}
      & & basic20 & 2 & 2 & -0.00017481256 & 0 & 2 & 2 & -0.00773612979 & 0 & 2 & 1 & -0.00206544273 & 1\\
      \cline{3-15}
      & & 2word16 & 3 & 3 & -0.00034446767 & 0 & 3 & 3 & -0.01310526071 & 0 & 3 & 3 & -0.01271757597 & 0\\
      \cline{3-15}
      & & basic16 & 4 & 6 & -0.01237917795 & 2 & 4 & 7 & -0.11203436164 & 3 & 4 & 4 & -0.11099256297 & 0\\
      \cline{3-15}
      & & 3class12 & 5 & 5 & -0.00946485322 & 0 & 5 & 5 & -0.01818160822 & 0 & 5 & 6 & -0.18384198515 & 1\\
      \cline{3-15}
      & & 2word12 & 6 & 7 & -0.01360245343 & 1 & 6 & 6 & -0.07942172914 & 0 & 6 & 5 & -0.17379245775 & 1\\
      \cline{3-15}
      & & comp8 & 7 & 4 & -0.00619759948 & 3 & 7 & 4 & -0.01573345733 & 3 & 7 & 7 & -0.21988288974 & 0\\
      \cline{3-15}
      & & basic12 & 8 & 8 & -0.16874098618 & 0 & 8 & 8 & -0.32090018785 & 0 & 8 & 8 & -0.44625701959 & 0\\
      \cline{2-15}
      & \multirow{8}{*}{\rotatebox{90}{Proportional}} & 3class16 & 1 & 1 & -0.15000000183 & 0 & 1 & 1 & -0.32803183792 & 0 & 1 & 2 & -0.45101422402 & 1\\
      \cline{3-15}
      & & basic20 & 2 & 3 & -0.22731830237 & 1 & 2 & 4 & -0.45407429983 & 2 & 2 & 1 & -0.45052415132 & 1\\
      \cline{3-15}
      & & 2word16 & 3 & 2 & -0.18899750304 & 1 & 3 & 3 & -0.4346028884 & 0 & 3 & 3 & -0.52489585375 & 0\\
      \cline{3-15}
      & & basic16 & 4 & 7 & -0.45303574889 & 3 & 4 & 7 & -0.579615909 & 3 & 4 & 4 & -0.57099747919 & 0\\
      \cline{3-15}
      & & 3class12 & 5 & 4 & -0.28309796453 & 1 & 5 & 2 & -0.33753384767 & 3 & 5 & 5 & -0.58017546055 & 0\\
      \cline{3-15}
      & & 2word12 & 6 & 6 & -0.31745131738 & 0 & 6 & 5 & -0.49108150848 & 1 & 6 & 7 & -0.61490864585 & 1\\
      \cline{3-15}
      & & comp8 & 7 & 5 & -0.2965234856 & 2 & 7 & 6 & -0.54963875987 & 1 & 7 & 8 & -0.65135140868 & 1\\
      \cline{3-15}
      & & basic12 & 8 & 8 & -0.47954187505 & 0 & 8 & 8 & -0.58639470743 & 0 & 8 & 6 & -0.59158613934 & 2\\
      \cline{2-15}
      & \multirow{8}{*}{\rotatebox{90}{Extraneous}} & 3class16 & 1 & 1 & -0.04210526403 & 0 & 1 & 1 & -0.1732211426 & 0 & 1 & 2 & -0.25848766731 & 1\\
      \cline{3-15}
      & & basic20 & 2 & 4 & -0.15048415667 & 2 & 2 & 3 & -0.2410656647 & 1 & 2 & 1 & -0.2478302857 & 1\\
      \cline{3-15}
      & & 2word16 & 3 & 2 & -0.05134151255 & 1 & 3 & 4 & -0.2463640901 & 1 & 3 & 3 & -0.29777195789 & 0\\
      \cline{3-15}
      & & basic16 & 4 & 6 & -0.17558403806 & 2 & 4 & 7 & -0.38191467167 & 3 & 4 & 4 & -0.40219971884 & 0\\
      \cline{3-15}
      & & 3class12 & 5 & 5 & -0.15869415661 & 0 & 5 & 2 & -0.22171184179 & 3 & 5 & 6 & -0.43333756896 & 1\\
      \cline{3-15}
      & & 2word12 & 6 & 7 & -0.18670016936 & 1 & 6 & 6 & -0.3512831245 & 0 & 6 & 5 & -0.42869639987 & 1\\
      \cline{3-15}
      & & comp8 & 7 & 3 & -0.15048415667 & 4 & 7 & 5 & -0.29031771829 & 2 & 7 & 7 & -0.4594561195 & 0\\
      \cline{3-15}
      & & basic12 & 8 & 8 & -0.35504148566 & 0 & 8 & 8 & -0.49858696195 & 0 & 8 & 8 & -0.53008440019 & 0\\
      \cline{2-15}
      & \multirow{8}{*}{\rotatebox{90}{Convergent}} & 3class16 & 1 & 7 & -1.33181526992 & 6 & 1 & 2 & -0.73706003039 & 1 & 1 & 5 & -0.84807451306 & 4\\
      \cline{3-15}
      & & basic20 & 2 & 8 & -1.65587234842 & 6 & 2 & 7 & -0.86310442053 & 5 & 2 & 8 & -0.90303209873 & 6\\
      \cline{3-15}
      & & 2word16 & 3 & 6 & -1.33177869336 & 3 & 3 & 5 & -0.79623023624 & 2 & 3 & 7 & -0.89905475536 & 4\\
      \cline{3-15}
      & & basic16 & 4 & 5 & -1.02369206677 & 1 & 4 & 6 & -0.85713632354 & 2 & 4 & 3 & -0.79663046993 & 1\\
      \cline{3-15}
      & & 3class12 & 5 & 2 & -0.77450139244 & 3 & 5 & 1 & -0.66271940447 & 4 & 5 & 2 & -0.77997709357 & 3\\
      \cline{3-15}
      & & 2word12 & 6 & 3 & -0.82018732762 & 3 & 6 & 3 & -0.74833314449 & 3 & 6 & 4 & -0.83475601093 & 2\\
      \cline{3-15}
      & & comp8 & 7 & 4 & -0.87004936668 & 3 & 7 & 8 & -0.92869922291 & 1 & 7 & 6 & -0.84854866977 & 1\\
      \cline{3-15}
      & & basic12 & 8 & 1 & -0.77238736541 & 7 & 8 & 4 & -0.77957401152 & 4 & 8 & 1 & -0.73119269609 & 7\\
      \hline
    \end{tabular}
  }
    \caption{Policy rankings under different reselection modes}
    \label{tab:comp}
  \end{table}
  \end{landscape}
